# Supplementary material for: Generic and Trend-aware Curriculum Learning for Relation Extraction in Graph Neural Networks
Source: arXiv:2205.08625 source file (2022-06-08)
Supplement: Supplementary file 1 [file additional_results.tex]

\begin{table*}[t]\small
    \centering
    \begin{tabular}{|l|l|l|l|l|l|l|l|}
\hline
 {\bf Additional Features} & {\bf Initial Embeddings}  & \multicolumn{3}{c}{{\bf GDPR}} & \multicolumn{3}{|c|}{{\bf PGR}}\\ \hline
 & & {\bf Precision} & {\bf Recall} & {\bf F1} & {\bf Precision} & {\bf Recall} & {\bf F1} \\ \hline
 \multirow{3}{*}{No} & Random & 32.09 & 41.17 & 36.07 & 81.70 &89.33  &85.35 \\
 & BioBERT &46.42 &02.06 & 03.95& 80.82 & 78.66 & 79.72\\
 & Doc2Vec  &72.93 & 35.00 & 47.00   & 83.54 & 88.00 & 85.71 \\ \hline
 \multirow{3}{*}{Yes} & Random & 64.71& \textbf{72.01} & 68.17 & 82.71 & \textbf{89.33} &85.89 \\
 & BioBERT & 73.99 & 52.46 &  61.39 & 86.95 & 80.00 & 83.33\\
 & Doc2Vec & \textbf{76.86} & 70.27& \textbf{73.42} & \textbf{86.84} & 88.00 & \textbf{87.41}\\ \hline
\end{tabular}
\caption{Effect of initial node embeddings and additional textual features using graph neural network on predicting causality between gene-disease/phenotype.}
%\nidhi{Here, no additional features with initial embeddings will be considered as GrapgSAGE?? }
%\hadi{yes and no, I think it's fine to keep this table as it is; it's important to know your model's performance with and w/o additional features.}
\label{ablation_study}
\end{table*}

\begin{table*}[!h]\small
    \centering
    \begin{tabular}{|l|c|c|c|c|c|c|c|c|c|} \hline
    {\bf Model} &  \multicolumn{3}{c}{{\bf GDPR} (Gene-Disease)} & \multicolumn{3}{|c|}{{\bf GDPR} (Gene-Phenotype)} & \multicolumn{3}{|c|}{{\bf PGR} (Gene-Phenotype)} \\ \hline
    & {\bf Precision} & {\bf Recall} & {\bf F1} & {\bf Precision} & {\bf Recall} & {\bf F1} & {\bf Precision} & {\bf Recall} & {\bf F1} \\ \hline
    %{\bf All ones} & 50.00 & 100.00 & 66.66 & -- & -- & --\\ \hline
    {\bf Co-occurrence} & 50.00 & 100.00 & 66.66 & 50.00 & 100.00 & 66.66 & 47.46 & 100.00 & 64.37 
     \\ \hline
    {\bf Relevance score} & 83.57 & 58.98 & 69.09 &52.06  & 06.48 & 11.53 & 72.73 & 21.33  & 32.99 
      \\ \hline
    %{\bf BoLSTM} & -- & -- & --& & & \\ \hline
    {\bf BioBERT} & 63.87 & 59.30 &61.50 & 76.86 & 73.87 & 75.33 & 81.82  & 72.00 &  76.60
    \\ \hline
    {\bf GraphSAGE+Doc2Vec} &72.93 & 35.00 & 47.00 & 81.84 & 84.71 & 83.25  & 83.54 & 88.00 &  85.71
     \\\hline
    \hline
    {\bf \SYSNAME} & 76.86 & 70.27 & {\bf 73.42$^$*} & 82.67 & 86.10 & {\bf84.35$^$*} & 86.84 & 88.00 & {\bf 87.41$^$*} 
      \\ \hline
    \end{tabular}
    \caption{Performance of different models on relation prediction for GDPR and PGR dataset. For a fair comparison for bench-marking, we evaluated gene-phenotype relations present in the GDPR graph using existing PGR dataset as it has been used before and gene-phenotypes pairs present in PGR  overlaps  with GDPR. 
    %\hadi{swap columns 2\&3}
    %\nidhi{\SYSNAME{} significantly outperforms BioBERT with p-value < 1\% and GraphSAGE with p-value <2\%.}
    %\hadi{need to include All Ones results for PGR.} \nidhi{that  would be same as Co-occurrence score, as that considers all the extracted pairs as positive}\hadi{how about removing all ones then and only including co-occurrence? for GDPR all will be labeled as non-causal, so p would be .5 and recall 1.}
    }
    %\hadi{should we call {\bf \SYSNAME{} w/o add. features} GraphSage and use it as a baseline to illustrate we have good baselines?}
    %\hadi{Reviewers may ask why don't you report results on GDPR (Gene-Phenotype)... perhaps we could say we resort to PGR for that task..}
    %\nidhi{(p-value < 1 \% for BioBERT, p < 2 \% for GraphSAGE) } 
    \label{performance}
\end{table*}
