# Supplementary material for: Generic and Trend-aware Curriculum Learning for Relation Extraction in Graph Neural Networks
Source: arXiv:2205.08625 source file (2022-06-08)
Supplement: Supplementary file 2 [file supplementry.tex]

\setcounter{figure}{0}    
\section{In-domain embeddings improves the  performance}

For these experiments, we re-train our model without additional textual feature but with different embedding initialization. As shown in Figure \ref{fig:ablation_w_feature} and \ref{fig:ablation_wo_feature}, Doc2Vec embeddings result in an overall better performance than BioBERT and random initialization approaches across the datasets. We attribute this result to in-domain training using text summaries of genes, diseases and phenotypes associated to rare diseases. In addition, the performance using BioBERT embeddings is considerably lower than that of other embeddings including Random. This is perhaps due to pre-training of BioBERT using a large scale PubMED dataset, which has a significantly lower prevalence of publications on rare vs. common diseases. On the other hand, we directly optimize Doc2Vec on in the domain datasets, which leads to higher performance of the model. We tried to fine tune BioBERT on our corpus but as the textual summaries were long, only few initial sentences were considered rest were discarded. Hence we focus on fine tuning Doc2Vec. 

\section{Additional Features improves the performance}

For these experiments, we re-train our models and include additional feature (i.e., relevance scores for \gdpr~and sentence embeddings for \pgr), with different node embedding initialization. 
Figure \ref{fig:ablation_w_feature} show that additional features improve the F1-scores of our model across all datasets and embedding initialization. 
These results show that both textual features and information obtained from graph structure contribute to predicting relations between nodes. 

\begin{figure}[t]
    \centering
    \includegraphics[scale=0.42]{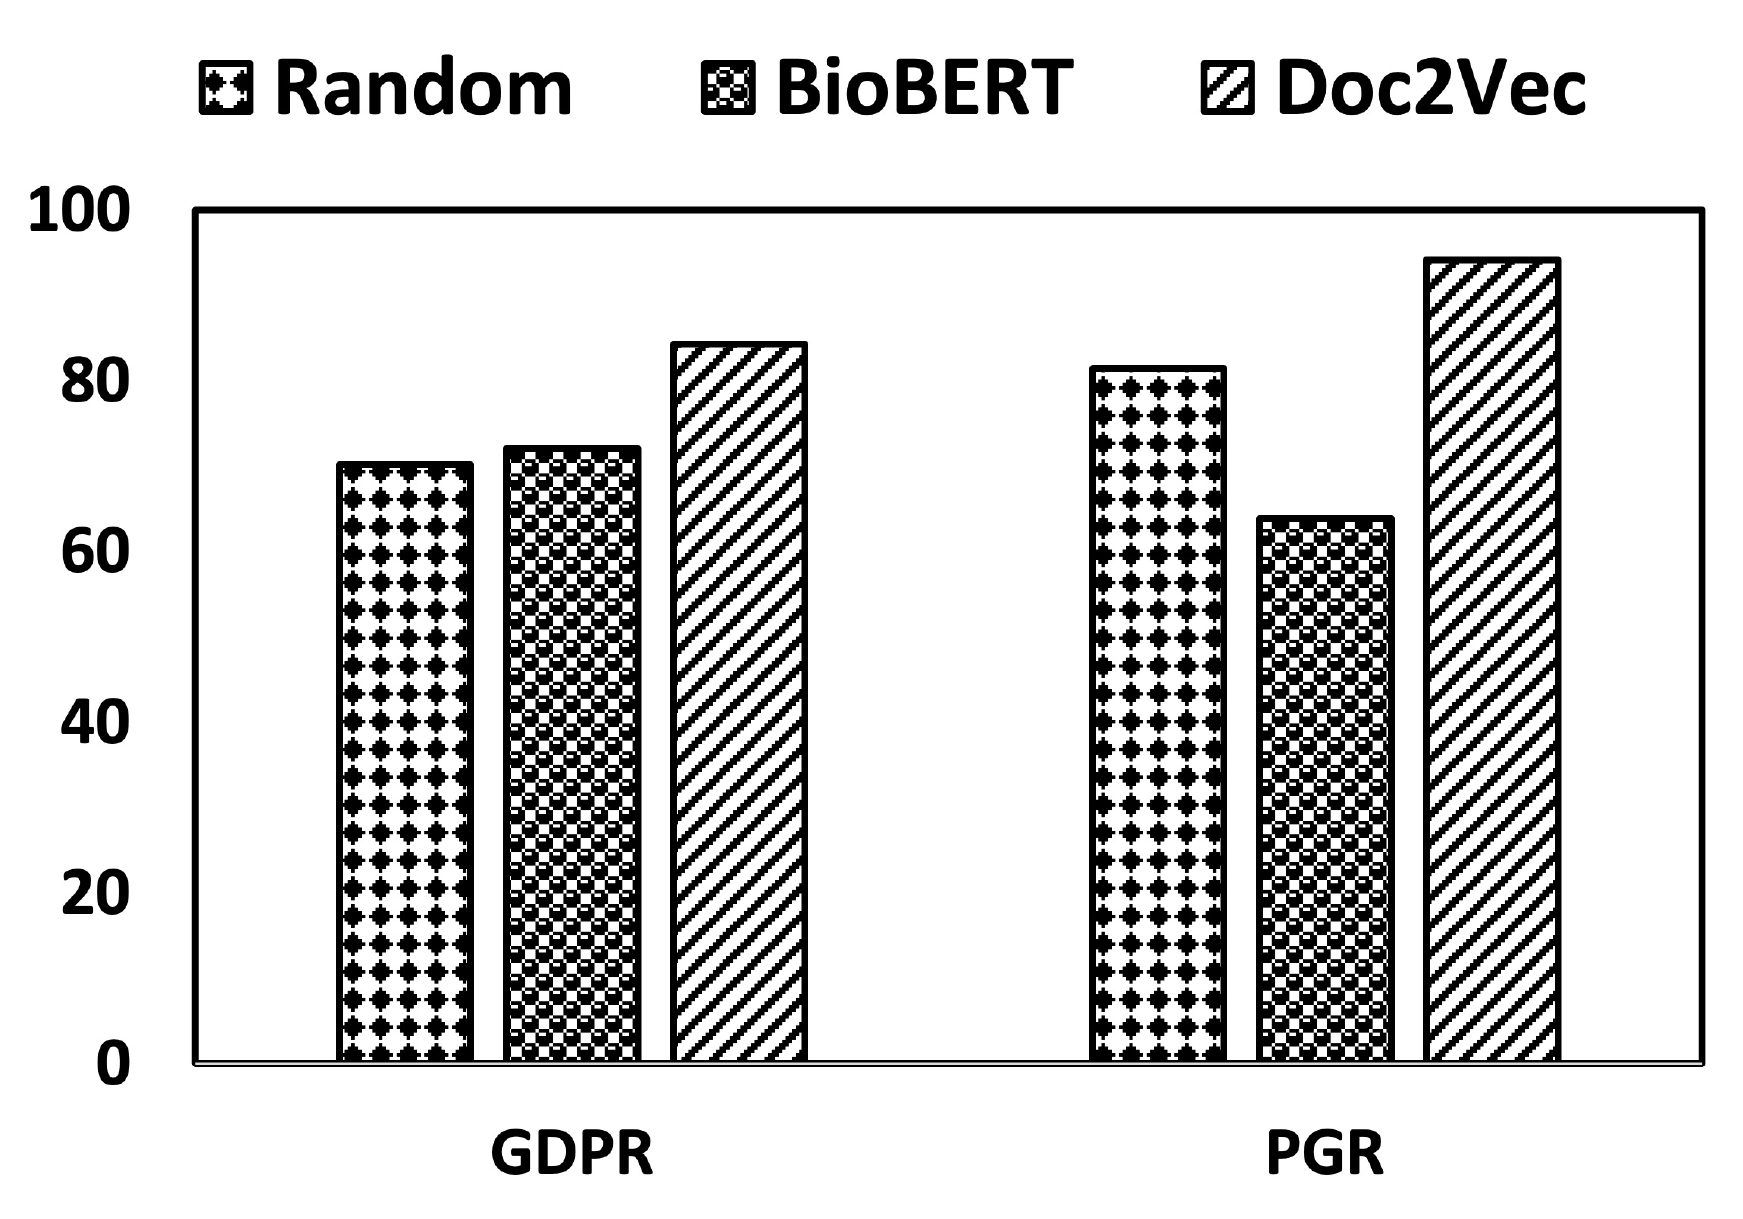}
    \caption{Performance of \gtnn{}  with Trend-SL with additional features.}
    \label{fig:ablation_w_feature}
\end{figure}
\begin{figure}[t]
    \centering
    \includegraphics[scale=0.42]{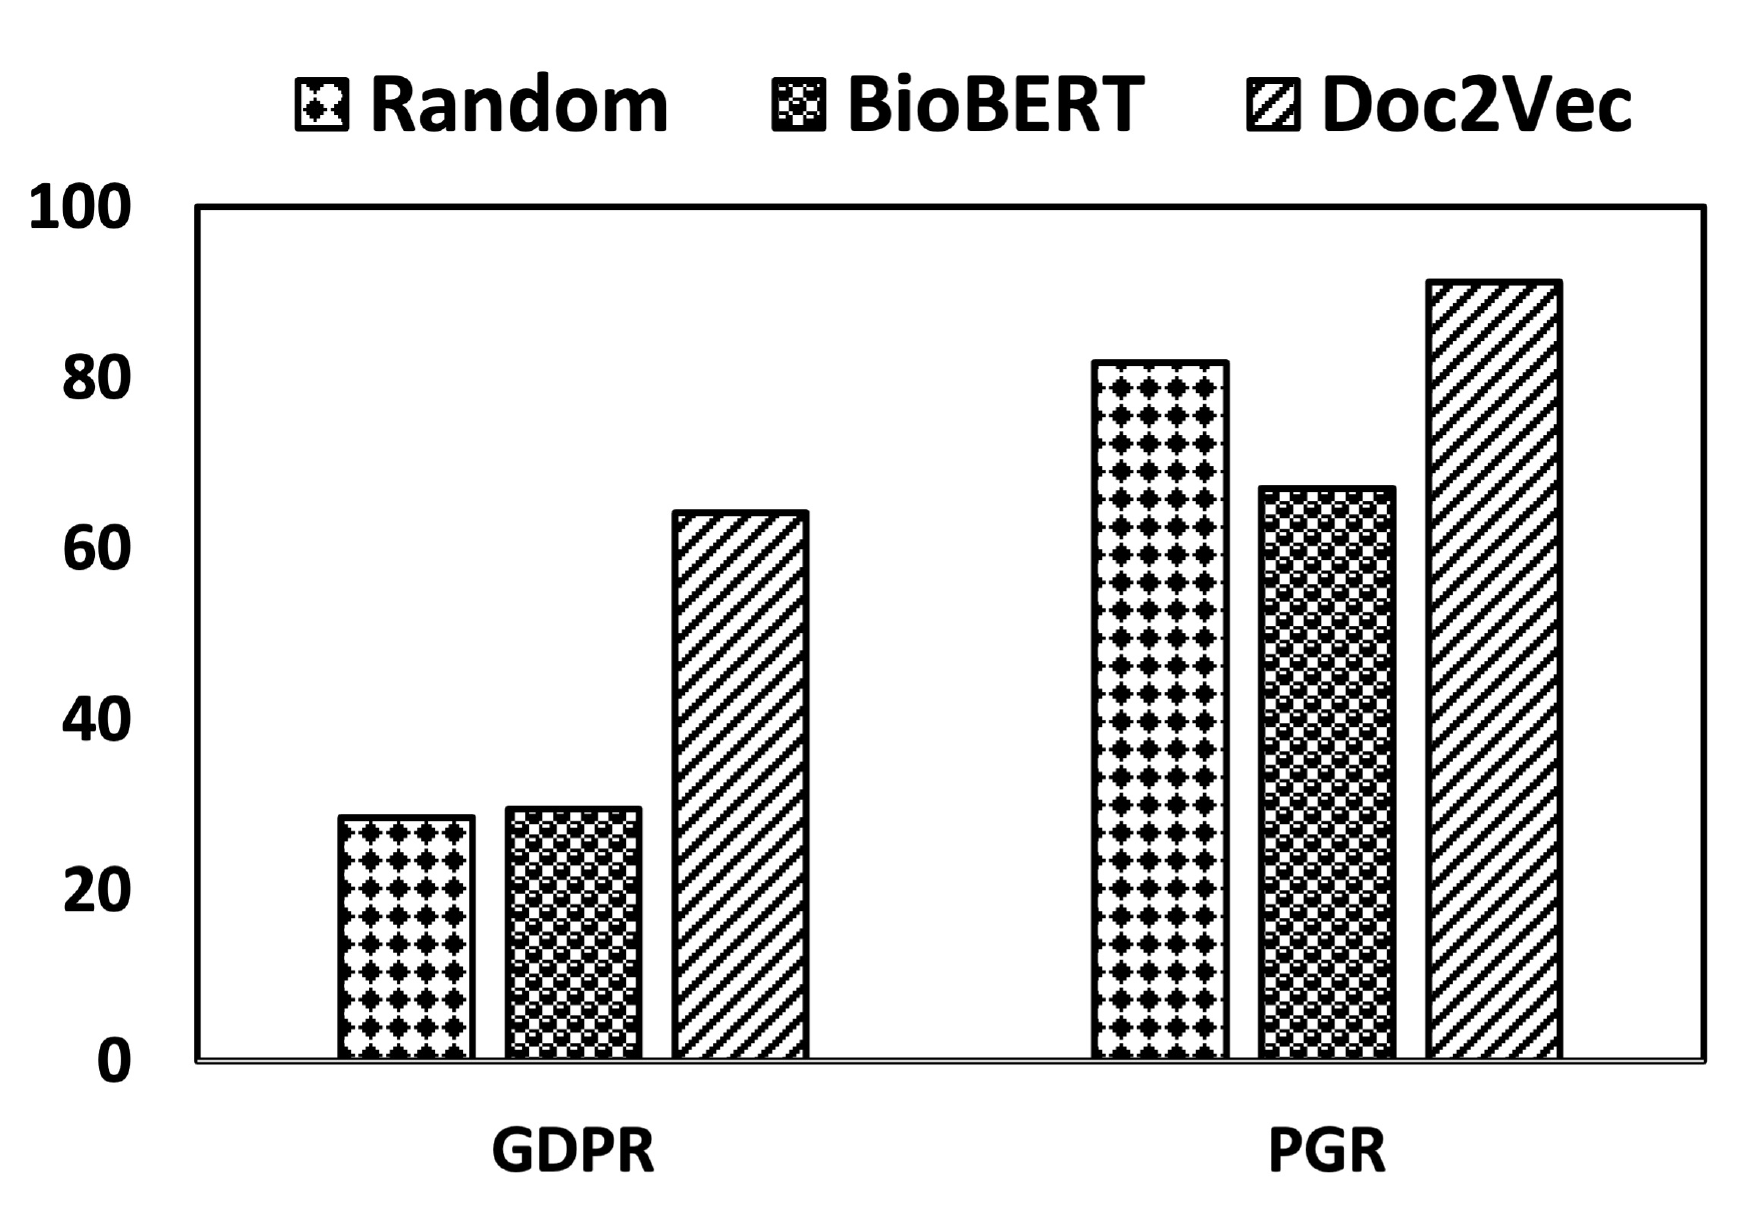}
    \caption{Performance of \gtnn{}  with Trend-SL without additional features.}
    \label{fig:ablation_wo_feature}
\end{figure}

\section{Inversions occur with falling or rising loss trends}
\begin{figure*}[!t]
    \centering
    \subfigure{\includegraphics[scale=0.45]{images/easy_fraction_analysis_1d 3.pdf}\label{fig:e2h_fraction_1d}}
    \subfigure{\includegraphics[scale=0.45]{images/hard_fraction_analysis_1d 2.pdf}\label{fig:h2e_fraction_1d}}
    \caption{Inversion heatmap of the examples when easy example converts to hard example (left) and vice versa (right)}
    \label{fig:fraction1d}
\end{figure*} 
Fig \ref{fig:fraction1d} shows the inversion heatmap for Easy-to-Hard and Hard-to-Easy for consecutive epoch where the y-axis fraction indicates the number of examples that were considered easy at epoch $e$ and had a rising trend which were converted into hard examples at epoch $e+1$. Similarly for Hard-to-Easy inversion heatmap. In Hard-to-Easy inversion the examples were hard at current epoch but had falling trend to eventually be inverted to easy examples. The area under the curve for Easy-to-Hard with rising trend is 24.87 and 4.51 for Hard-to-Easy.
